# Supplementary material for: Optimal coarse-grained site selection in elastic network models of biomolecules
Source: arXiv:1806.06804 ancillary file (2018-12-11)
Supplement: Supplementary file 1 [file supp_info.pdf]

# Supplementary information to Optimal coarse-grained site selection in elastic network models of biomolecules

Patrick Diggins IV,<sup>1</sup> Changjiang Liu,<sup>1,2</sup> Markus Deserno,<sup>1</sup> and Raffaello Potestio<sup>3,4,\*</sup>

<sup>1</sup>*Department of Physics, Carnegie Mellon University, Pittsburgh, PA 15213, USA*

<sup>2</sup>*Department of Biophysics, University of Michigan, Ann Arbor, MI 48109, USA*

<sup>3</sup>*Physics Department, University of Trento, via Sommarive, 14 I-38123 Trento, Italy*

<sup>4</sup>*INFN-TIFPA, Trento Institute for Fundamental Physics and Applications, I-38123 Trento, Italy*

## I. EFFICIENT SCHEME FOR HESSIAN MATRIX INVERSION

In the process of optimising the model efficiency, e.g. looking for the selection of atoms providing the lowest average eigenvalue ratio  $f_a$ , the computational bottleneck consists in the inversion of the Hessian matrix of the particles that we want to remove in a given step. Luckily, one does not need to invert the entire interaction matrix when making a single MC step, because it is possible to make use of information from the previous step. Since only one particle is being replaced, it is sufficient to change three rows and three columns of the removed Hessian matrix  $\mathbf{H}_B$ , and employ information from the calculation of the inverse for the previous  $\mathbf{H}_B$  to quickly calculate the new inverse. The first step is to calculate the inverse matrix of the atoms that are the same for both reductions. Let us call this group of atoms  $S$ , the previously removed atom that is now not removed  $O$ , and the new atom to be removed  $N$  ( $S$  for same,  $O$  for old, and  $N$  for new). One can write the original sub-Hessian of removed atoms  $\mathbf{H}_{B,0}$  as:

$$\mathbf{H}_{B,0} = \begin{pmatrix} \mathbf{H}_O & \mathbf{H}_{O,S} \\ \mathbf{H}_{O,S}^\dagger & \mathbf{H}_S \end{pmatrix}, \quad (1)$$

where  $\mathbf{H}_{O,S}$  is the interaction matrix between atom  $O$  and the other atoms. The first goal is to find the inverse of  $\mathbf{H}_S$  because it will be useful later. One can partition the inverse of  $\mathbf{H}_B$  the same way:

$$\mathbf{H}_{B,0}^{-1} = \begin{pmatrix} \mathbf{M}_1 & \mathbf{M}_{1,2} \\ \mathbf{M}_{1,2}^\dagger & \mathbf{M}_2 \end{pmatrix}, \quad (2)$$

where  $\mathbf{M}_1$  has the same size and is in the same position in the inverse matrix as  $\mathbf{H}_O$  is in the original matrix. The inverse of  $\mathbf{H}_S$  is [? ]:

$$\mathbf{H}_S^{-1} = \mathbf{M}_2 - \mathbf{M}_{1,2}^\dagger \mathbf{M}_1^{-1} \mathbf{M}_{1,2} \quad (3)$$

We define the new sub-Hessian of removed atoms  $\mathbf{H}_{B,1}$ ,

$$\mathbf{H}_{B,1} = \begin{pmatrix} \mathbf{H}_N & \mathbf{H}_{N,S} \\ \mathbf{H}_{N,S}^\dagger & \mathbf{H}_S \end{pmatrix}, \quad (4)$$

where  $\mathbf{H}_N$  is the Hessian sub-matrix for the new atom to be removed. For the sake of readability, we define  $\mathbf{N} = \mathbf{H}_N - \mathbf{H}_{N,S} \mathbf{H}_S^{-1} \mathbf{H}_{N,S}^\dagger$ . The inverse is then:

$$\mathbf{H}_{B,1}^{-1} = \begin{pmatrix} \mathbf{a} & \mathbf{b} \\ \mathbf{b}^\dagger & \mathbf{c} \end{pmatrix} \quad (5)$$

with:

$$\mathbf{a} = \mathbf{H}_N^{-1}$$

$$\mathbf{b} = -\mathbf{N}^{-1} \mathbf{H}_{N,S} \mathbf{H}_S^{-1}$$

$$\mathbf{c} = \mathbf{H}_S^{-1} + \mathbf{H}_S^{-1} \mathbf{H}_{N,S}^\dagger \mathbf{N}^{-1} \mathbf{H}_{N,S} \mathbf{H}_S^{-1}.$$

Thus, instead of having to take the inverse of a very large matrix, one just needs to find the inverse of two  $3 \times 3$  matrices, and perform some additional matrix multiplication and addition. This reduces the time needed to create a new reduction by orders of magnitude, however, over time numerical errors accumulate, and eventually the total error becomes appreciable. After a (problem-dependent) number of steps it is thus necessary to calculate the inverse matrix directly.

## II. FLUCTUATIONS

We report here the mean square fluctuations (MSF) of the atoms of adenylate kinase, Fig. 1, and the adenine riboswitch, Fig. 2. The reference for both molecules is the all-atom harmonic ENM, while for each relevant coarse-grained representation we report the MSF computed from the harmonic approximation of the corresponding ENM. For atom  $i$ , the MSF is computed according to the following expression:

$$MSF_i \equiv \langle |\Delta \mathbf{r}_i|^2 \rangle = \sum_{\mu=1}^3 (\mathbf{H}_{ii}^{\mu\mu})^{-1} \quad (6)$$

where  $\mathbf{H}$  is the hENM Hamiltonian and  $\mu$  is the Cartesian coordinate index.

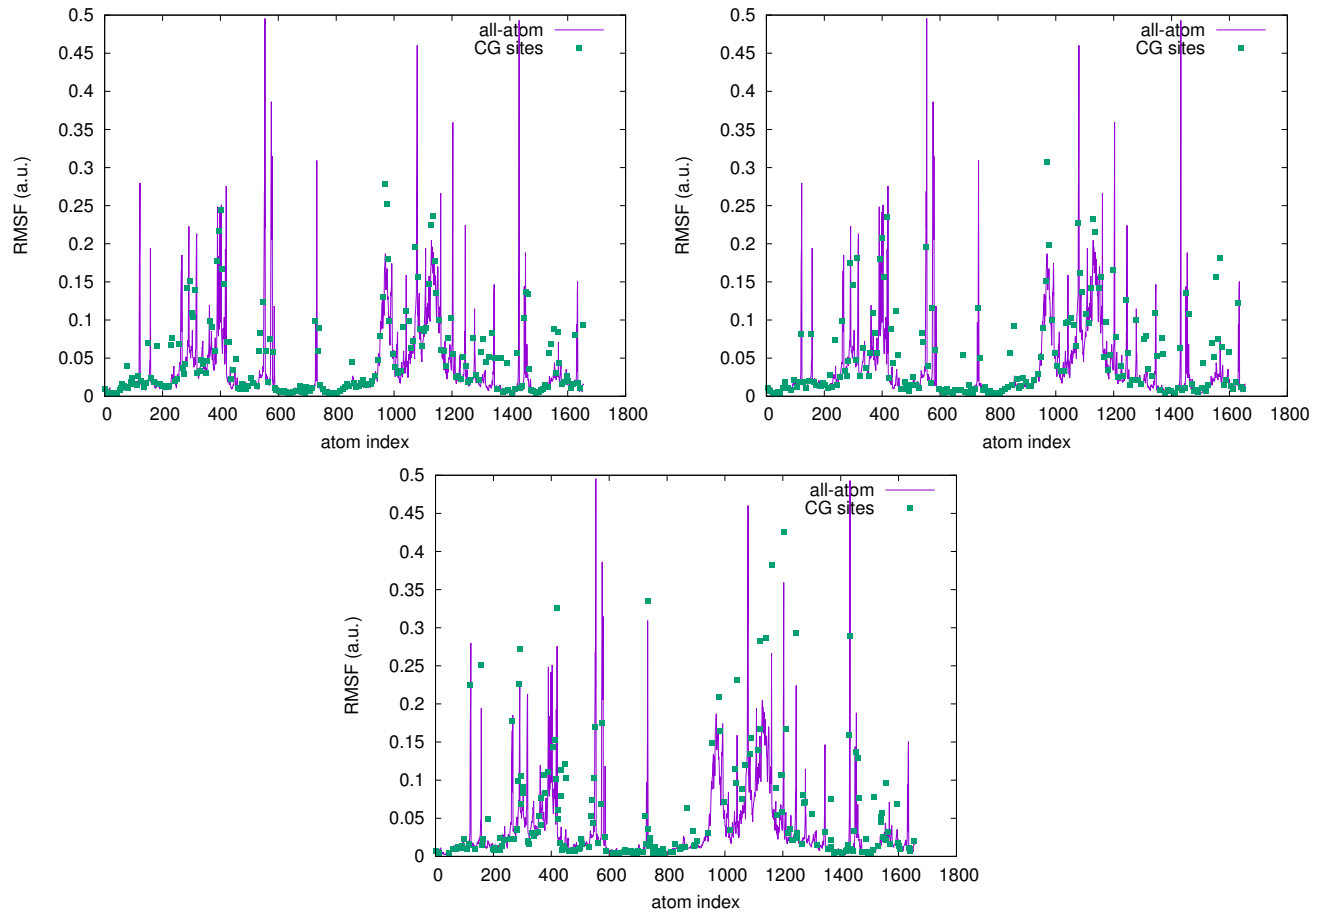

FIG. 1. Mean square fluctuations for adenylate kinase. In each plot the data obtained from the all-atom ENM are reported in purple. The data for the harmonic CG-ENM's are provided as green squared. Top left:  $C_\alpha$ -only model; top right:  $C_\beta$ -only model; bottom: optimised model.

---

\* [raffaello.potestio@unitn.it](mailto:raffaello.potestio@unitn.it)

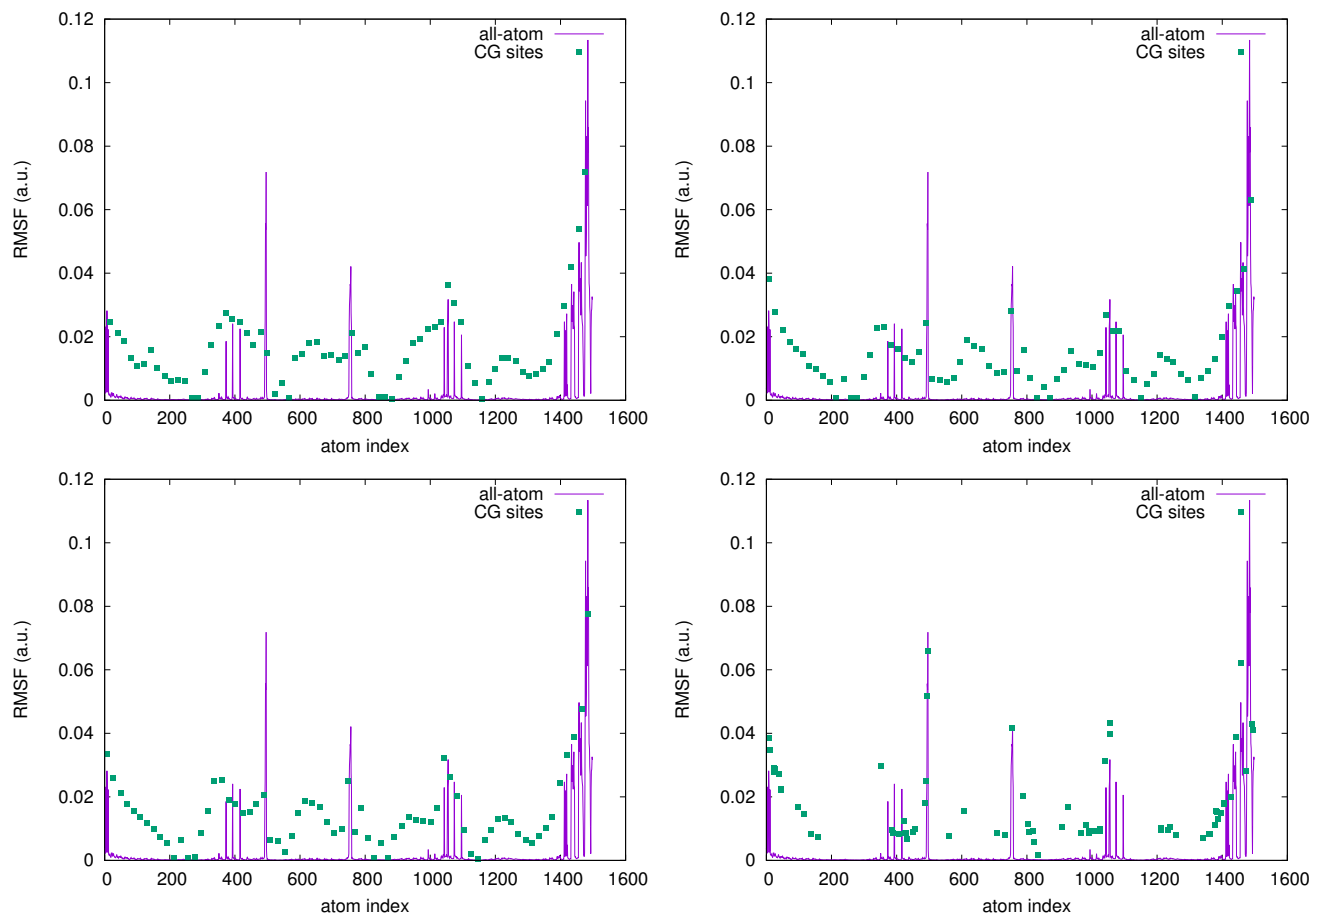

FIG. 2. Mean square fluctuations for adenine riboswitch. In each plot the data obtained from the all-atom ENM are reported in purple. The data for the harmonic CG-ENM's are provided as green squared. Top left: P-only model; top right: C1'-only model; bottom left: C2-only model; bottom right: optimised model.
